# Supplementary material for: Subtraction of temperature induced phase noise in the LISA frequency band
Source: arXiv:1302.5628 source file (2013-06-19)
Supplement: Supplementary file 1 [file appendix.tex]

\appendix

\section{Expressions for the conditioned spectral analysis \label{sec:condExpr}}

The recursive application of Eq.~\ref{eq.cond} leads to the following array of equations:
\begin{eqnarray}
 S_{\Phi \Phi \cdot T_{1}}(f)  &=& S_{\Phi \Phi}\,(1 - \gamma^2_{T_1 \Phi}) \nonumber \\
 S_{\Phi \Phi \cdot T_{2}!}(f) &=& S_{\Phi \Phi \cdot T_{1}}\,(1 - \gamma^2_{T_2 \Phi \cdot T_1}) \nonumber \\
 S_{\Phi \Phi \cdot T_{3}!}(f) &=& S_{\Phi \Phi \cdot T_{2}!}\,(1 - \gamma^2_{T_3 \Phi \cdot T_2}!) \nonumber \\
 S_{\Phi \Phi \cdot T_{4}!}(f) &=& S_{\Phi \Phi \cdot T_{3}!}\,(1 - \gamma^2_{T_4 \Phi \cdot T_3}!) \nonumber \\
\end{eqnarray} 

\martin{Is it really necessary to have an Appendix just for this? Looks a bit silly....}
